# Supplementary material for: Video Recognition in Portrait Mode
Source: arXiv:2312.13746 source file (2023-12-21)
Supplement: Supplementary file 1 [file suppl_duration_v2.pdf]

Average duration per category

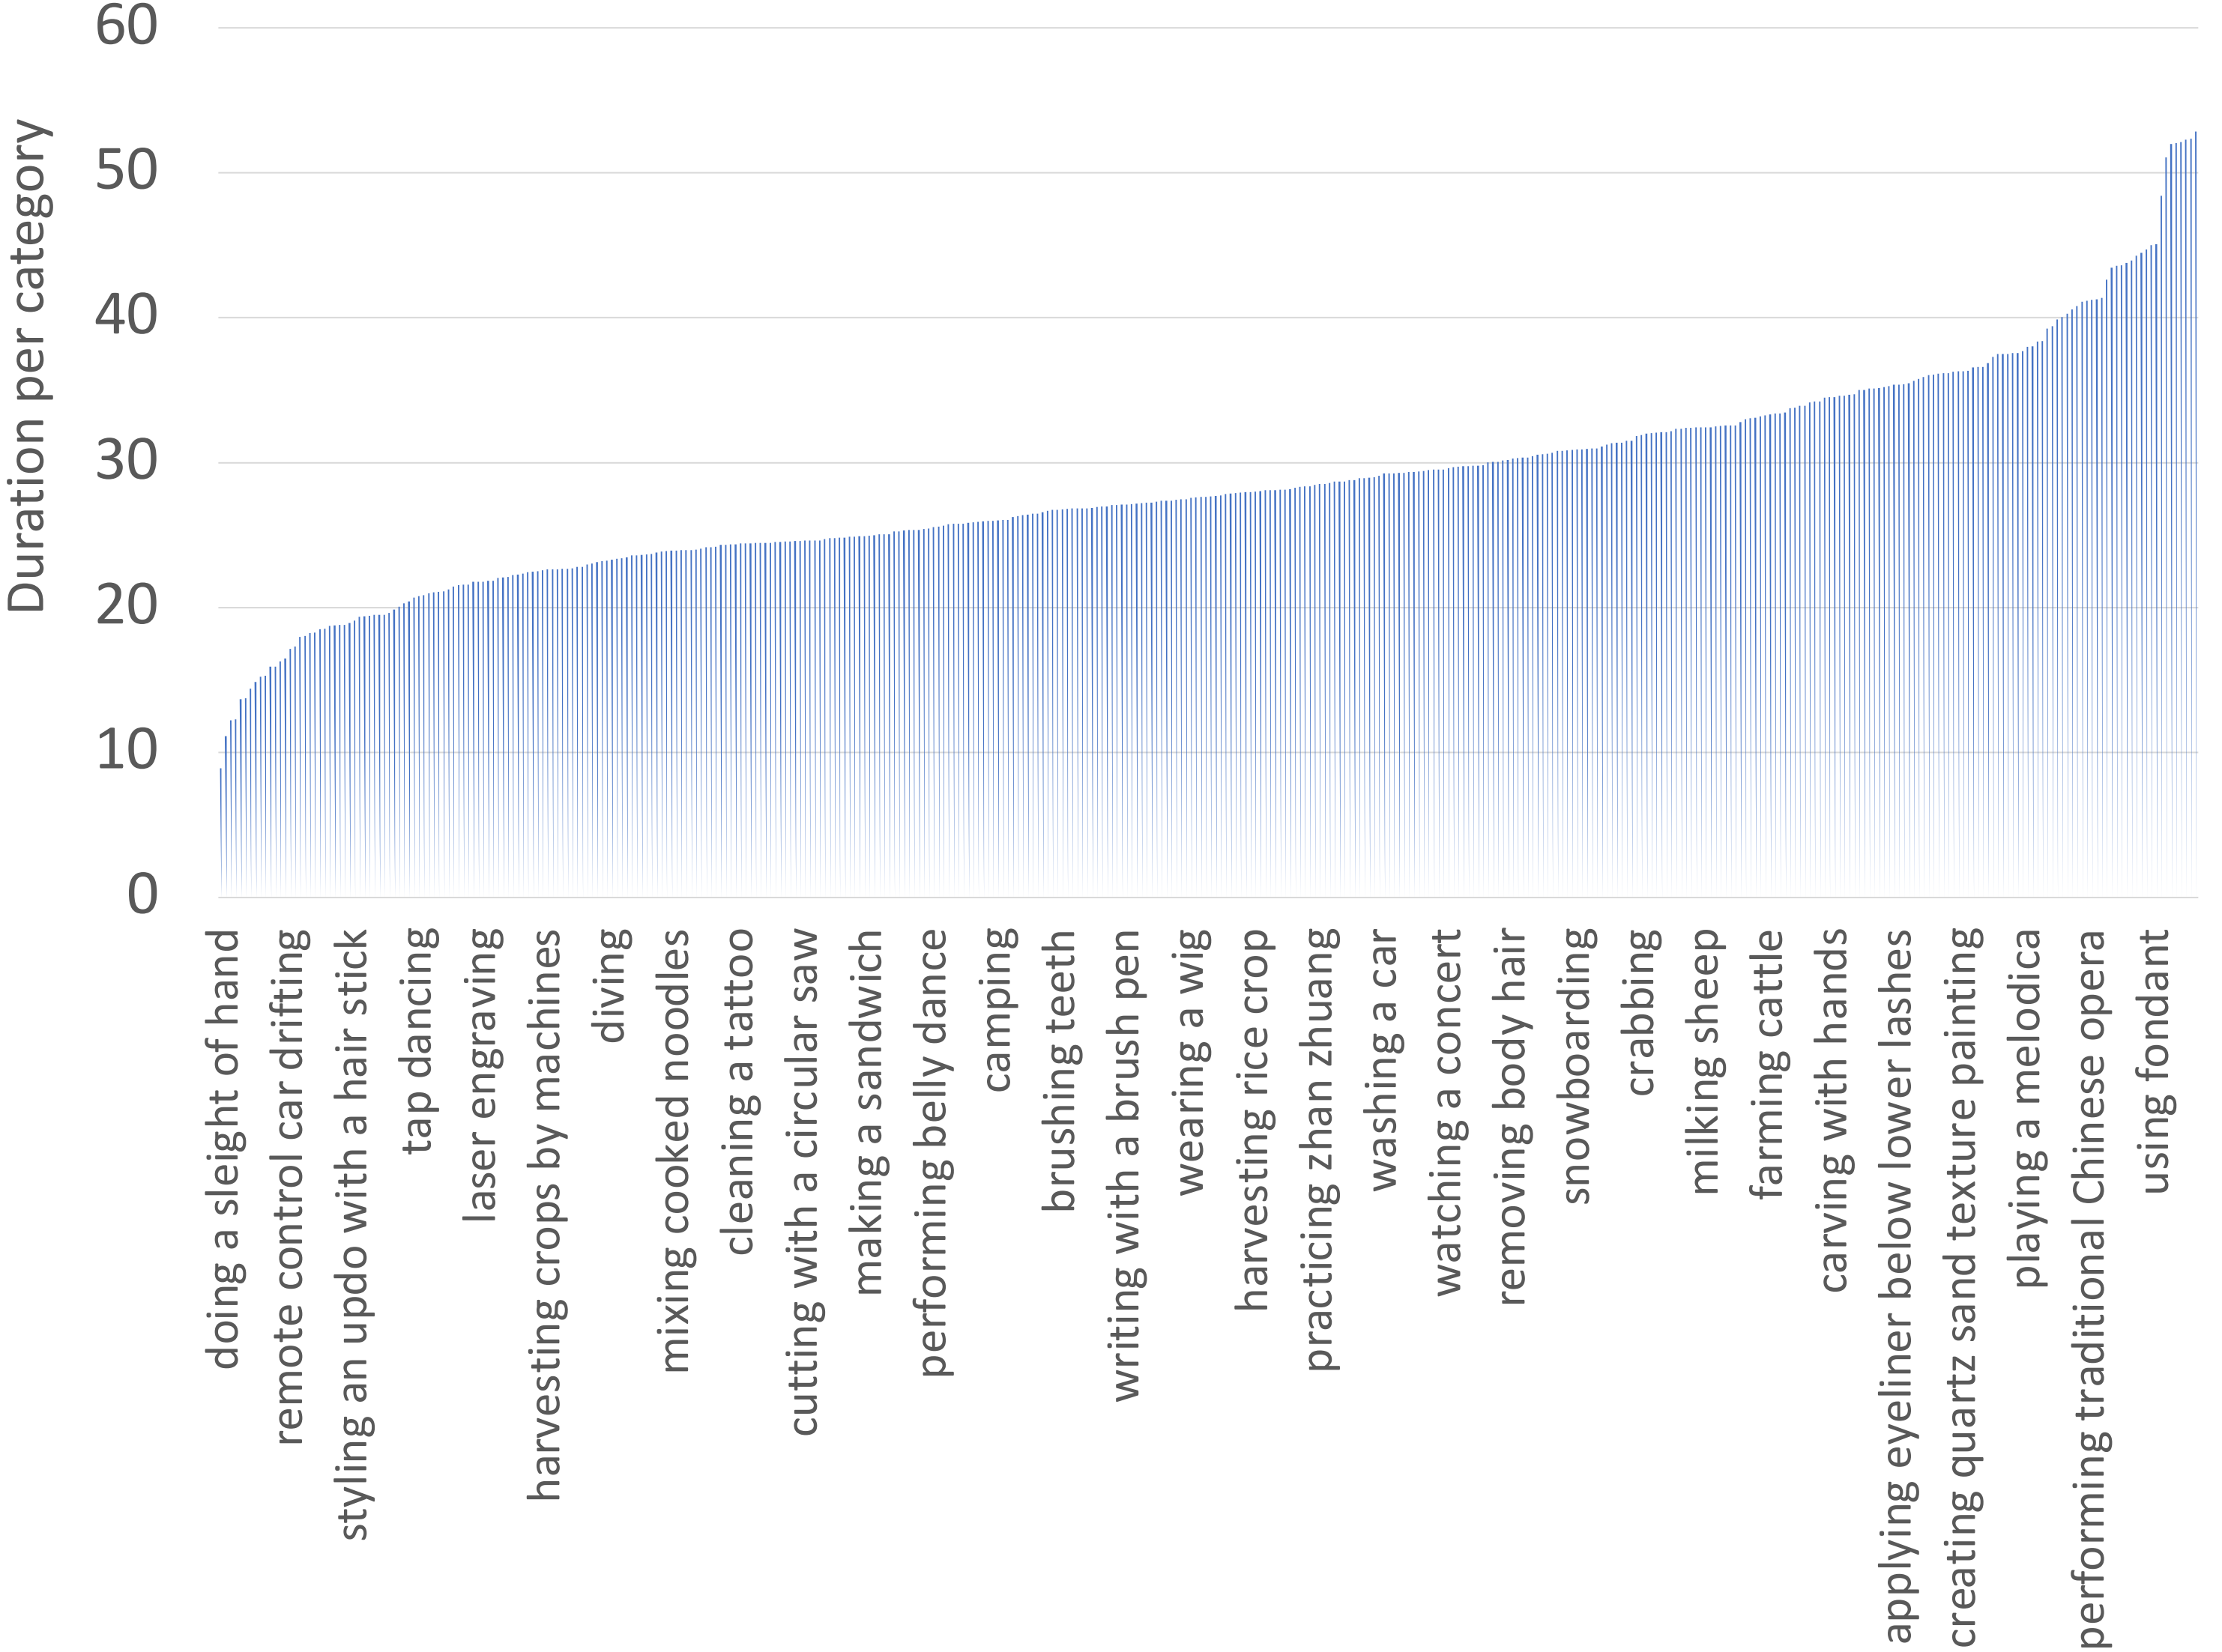

Average duration per category

Duration per category

50.00  
45.00  
40.00  
35.00  
30.00  
25.00  
20.00  
15.00  
10.00  
5.00  
0.00

- card magic with empty hands
- engrave on pencils
- disco dancing
- pedicure
- hugging
- laser welding
- fish soup
- lo mein
- make hand-crafted lanterns
- wrap book covers
- Tai chi
- stir-fried deep fried seafood
- knitting by needles
- ballet
- whistling
- clip eyelashes
- swimming
- white boiled shrimp
- making a fire lacquer seal
- playing mahjong games
- oil back massage
- applying the concealer
- knitting by hand
- stir-fried meat
- open mystery boxes
- street interview
