# Supplementary material for: Video Recognition in Portrait Mode
Source: arXiv:2312.13746 source file (2023-12-21)

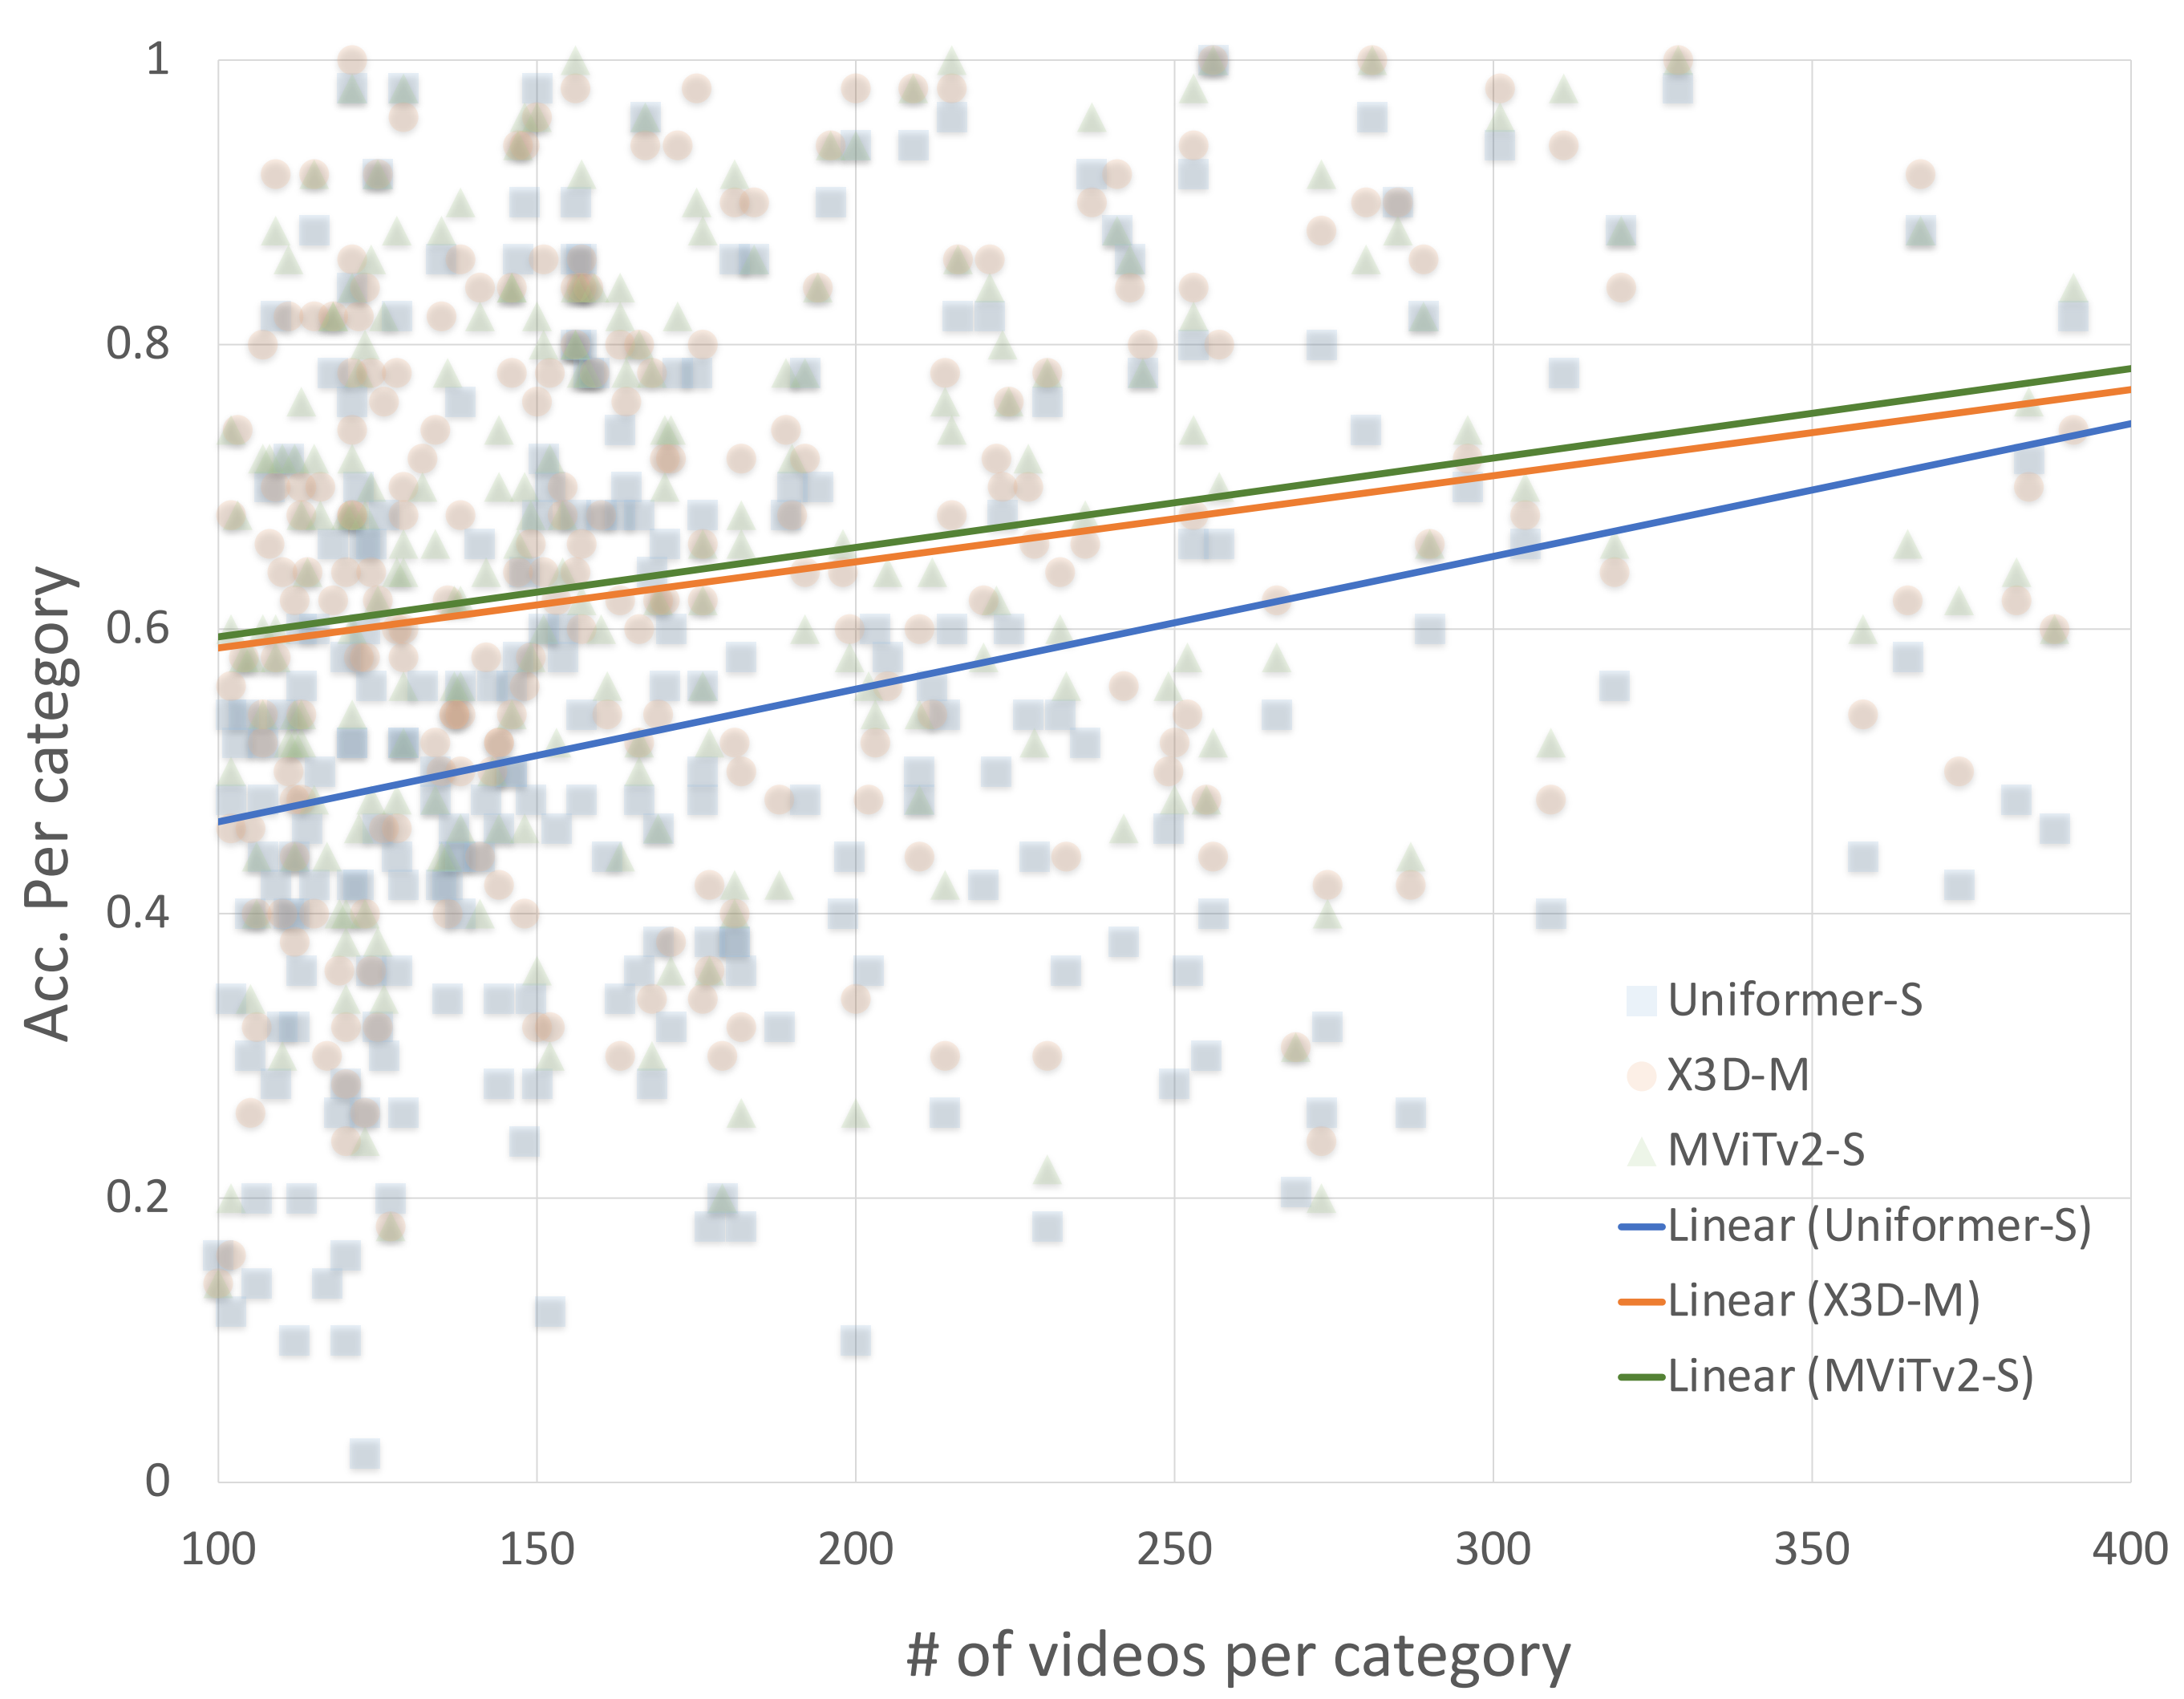

Acc. Per category

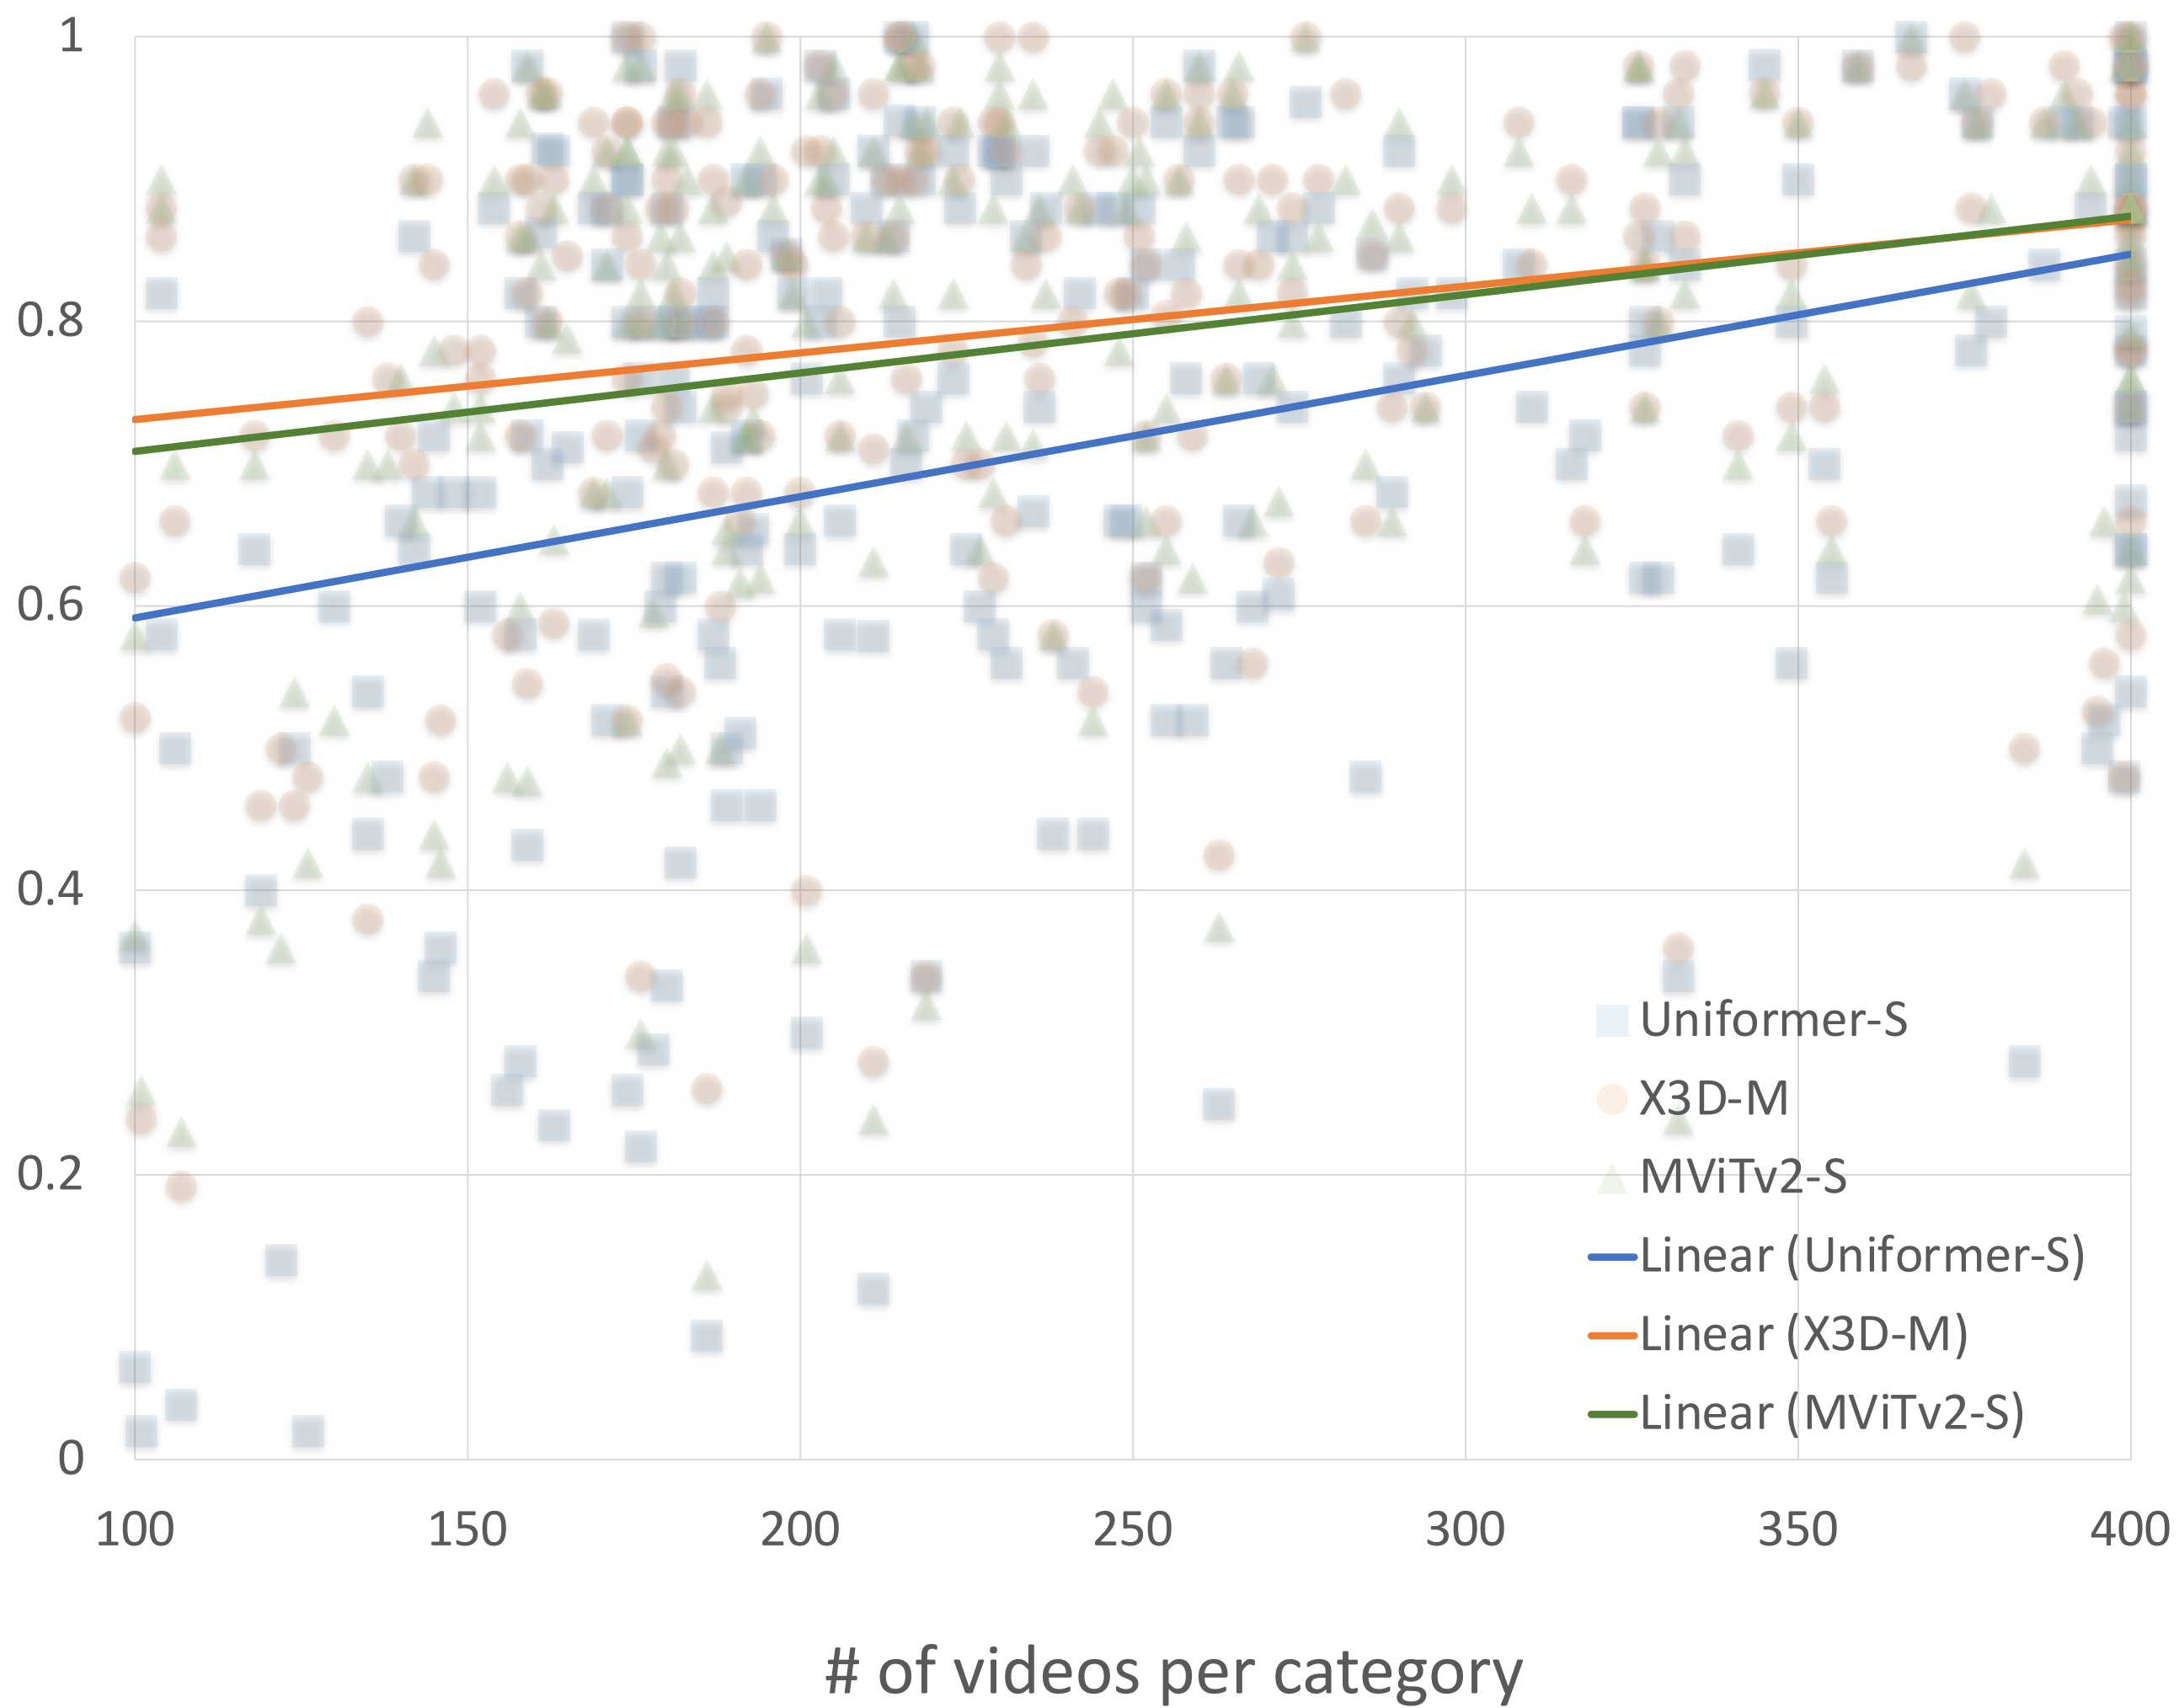

Supplement: Supplementary file 2 [file suppl_vcnt_acc.pdf]
